# Supplementary material for: Intrinsic process for upconversion photoluminescence via $K$-momentum phonon coupling in carbon nanotubes
Source: arXiv:2404.03849 ancillary file (2024-10-11)
Supplement: Supplementary file 1 [file SM_UpconversionPL.pdf]

# Supplemental Material for "Intrinsic process for upconversion photoluminescence via $K$-momentum phonon coupling in carbon nanotubes"

Daichi Kozawa,[1,2,3,*] Shun Fujii,[1,4] and Yuichiro K. Kato[1,2,†]

[1] *Quantum Optoelectronics Research Team, RIKEN Center for Advanced Photonics, Wako, Saitama 351-0198, Japan*

[2] *Nanoscale Quantum Photonics Laboratory, RIKEN Cluster for Pioneering Research, Wako, Saitama 351-0198, Japan*

[3] *Research Center for Materials Nanoarchitectonics, National Institute for Materials Science, Tsukuba, Ibaraki 305-0044, Japan*

[4] *Department of Physics, Faculty of Science and Technology, Keio University, Yokohama, Kanagawa 223-8522, Japan*

[*] Corresponding Author: kozawa.daichi@nims.go.jp

[†] Corresponding Author: yuichiro.kato@riken.jp

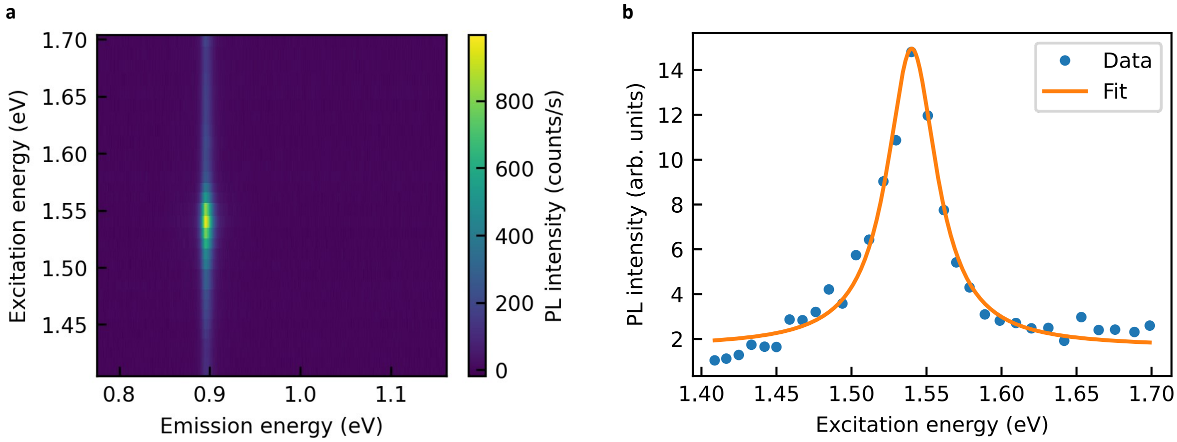


FIG. S1. (a) A PLE map and (b) a PLE spectrum of a (9,8) nanotube with an excitation power of 20 $\mu$W. Dots are experimental results and a line is a Lorentzian fit.

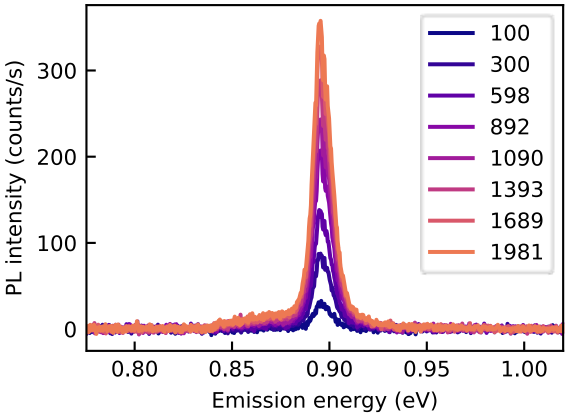


FIG. S2. Excitation power dependence of UCPL spectra with an excitation energy of 0.800 eV. The excitation powers are 100, 300, 598, 892, 1090, 1393, 1689, and 1981 $\mu$W from bottom to top as indicated in the legend.

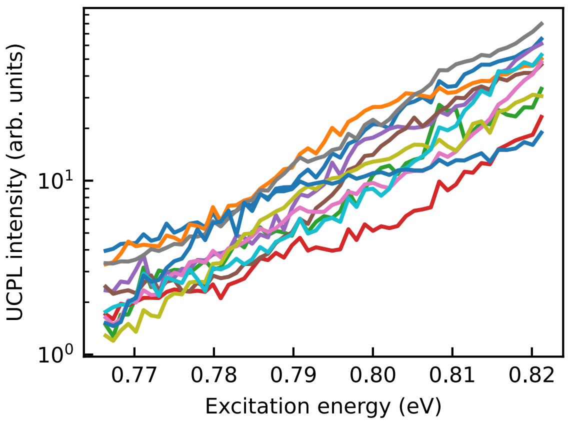


FIG. S3. UCPLE spectra for various (13,5) SWNTs with an excitation power of 1000 $\mu$W.

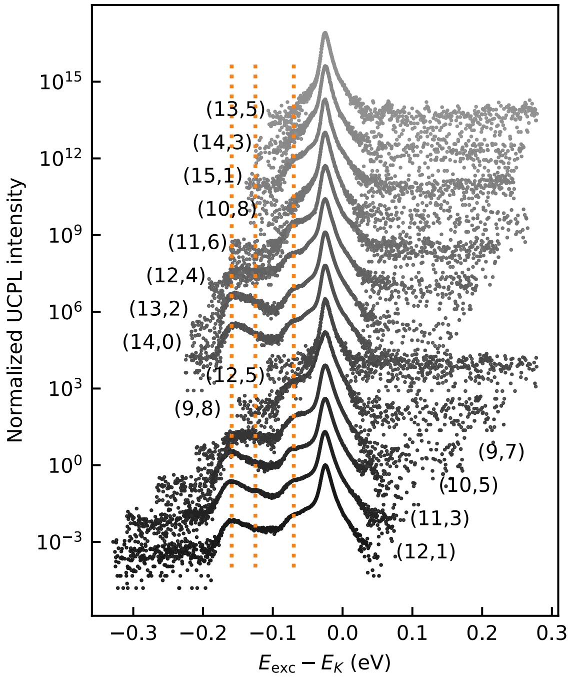


FIG. S4. PL spectra for the various chiralities with an excitation power of 10 $\mu$W. Vertical dotted lines indicate the energy differnce of 70, 125, and 159 meV. The spectra are displaced vertically for clarity.

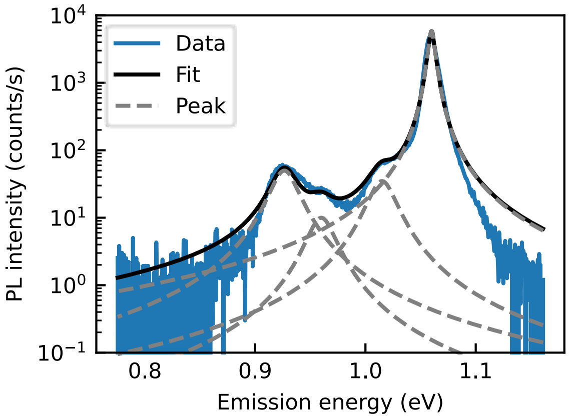


FIG. S5. PL spectrum for a (11,3) SWNT with an excitation energy of 1.60 eV and a power of 10 $\mu$W. A solid black curve is a fit using a tetra-Lorentzian function and broken lines are the individual components of the fit.

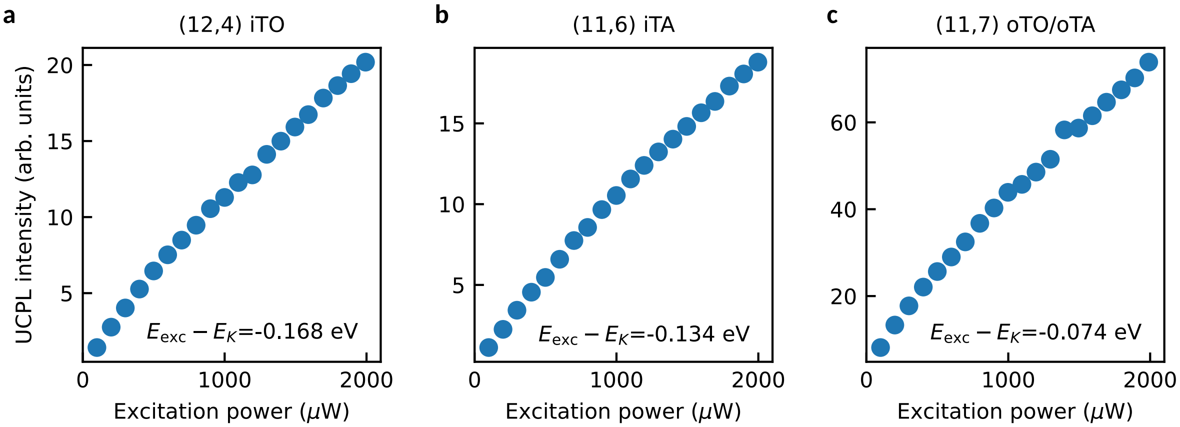


FIG. S6. Excitation power dependence of the UCPL intensity with an excitation energy of 0.800 eV involving the $K$-momentum (a) iTO phonon in a (12,4) SWNT, (b) iTA phonon in a (11,6) SWNT, and (c) oTO/oTA phonon in a (11,7) SWNT.
